# Supplementary material for: Aligning Offline Metrics and Human Judgments of Value for Code Generation Models
Source: arXiv:2210.16494 source file (2023-06-13)
Supplement: Supplementary file 1 [file appendix.tex]

\section{Appendices}

\begin{figure*}
    \centering
    \includegraphics[width=\linewidth]{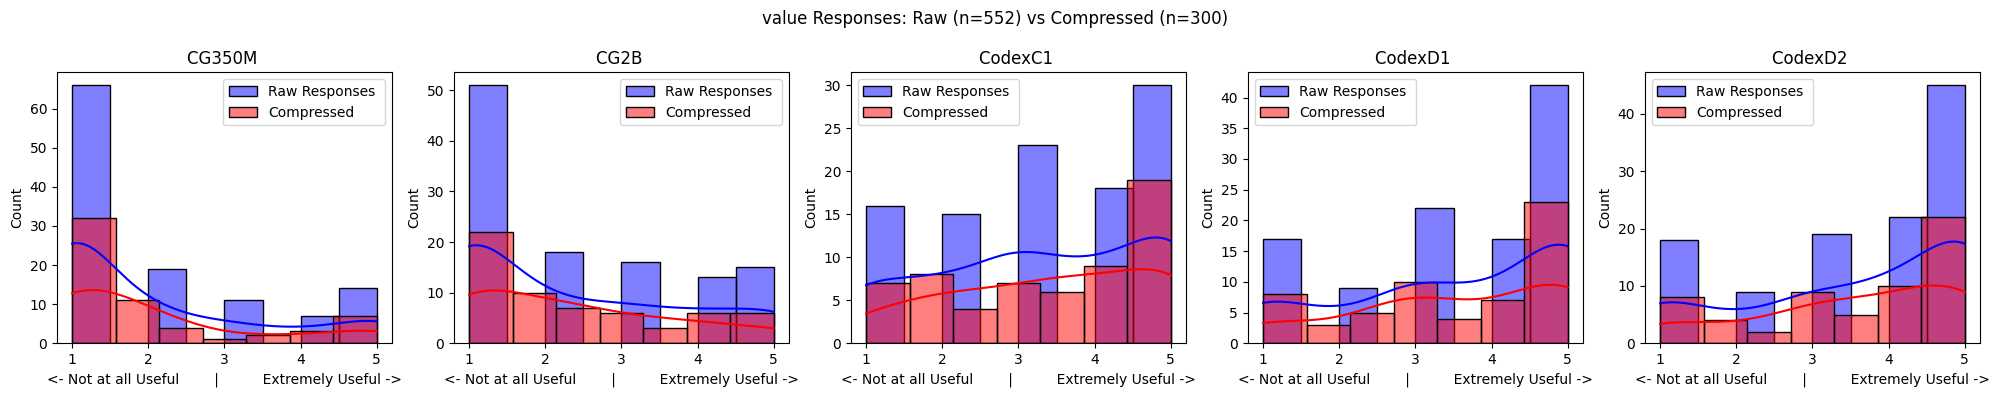}
    \caption{Distribution of participant perception of value of code suggestions (Likert scale) for five state-of-the-art code generation models. The survey asked {\em Assuming you were a programmer writing a solution to the task, and you received snippet A ... how useful will this be to you?} 
    \gagan{Fix size convert into box plot and make it similar to the box plot figure from the offline experiments. Saleema: Box plots aren't advised for ordinal data. The closest thing to get a similar shape for comparison is a diverging bar chart. I tried this in Fig 9. Let's discuss.}
    }
    \label{fig:my_label}
\end{figure*}

\begin{figure}
    \centering
    \includegraphics[width=0.3\linewidth]{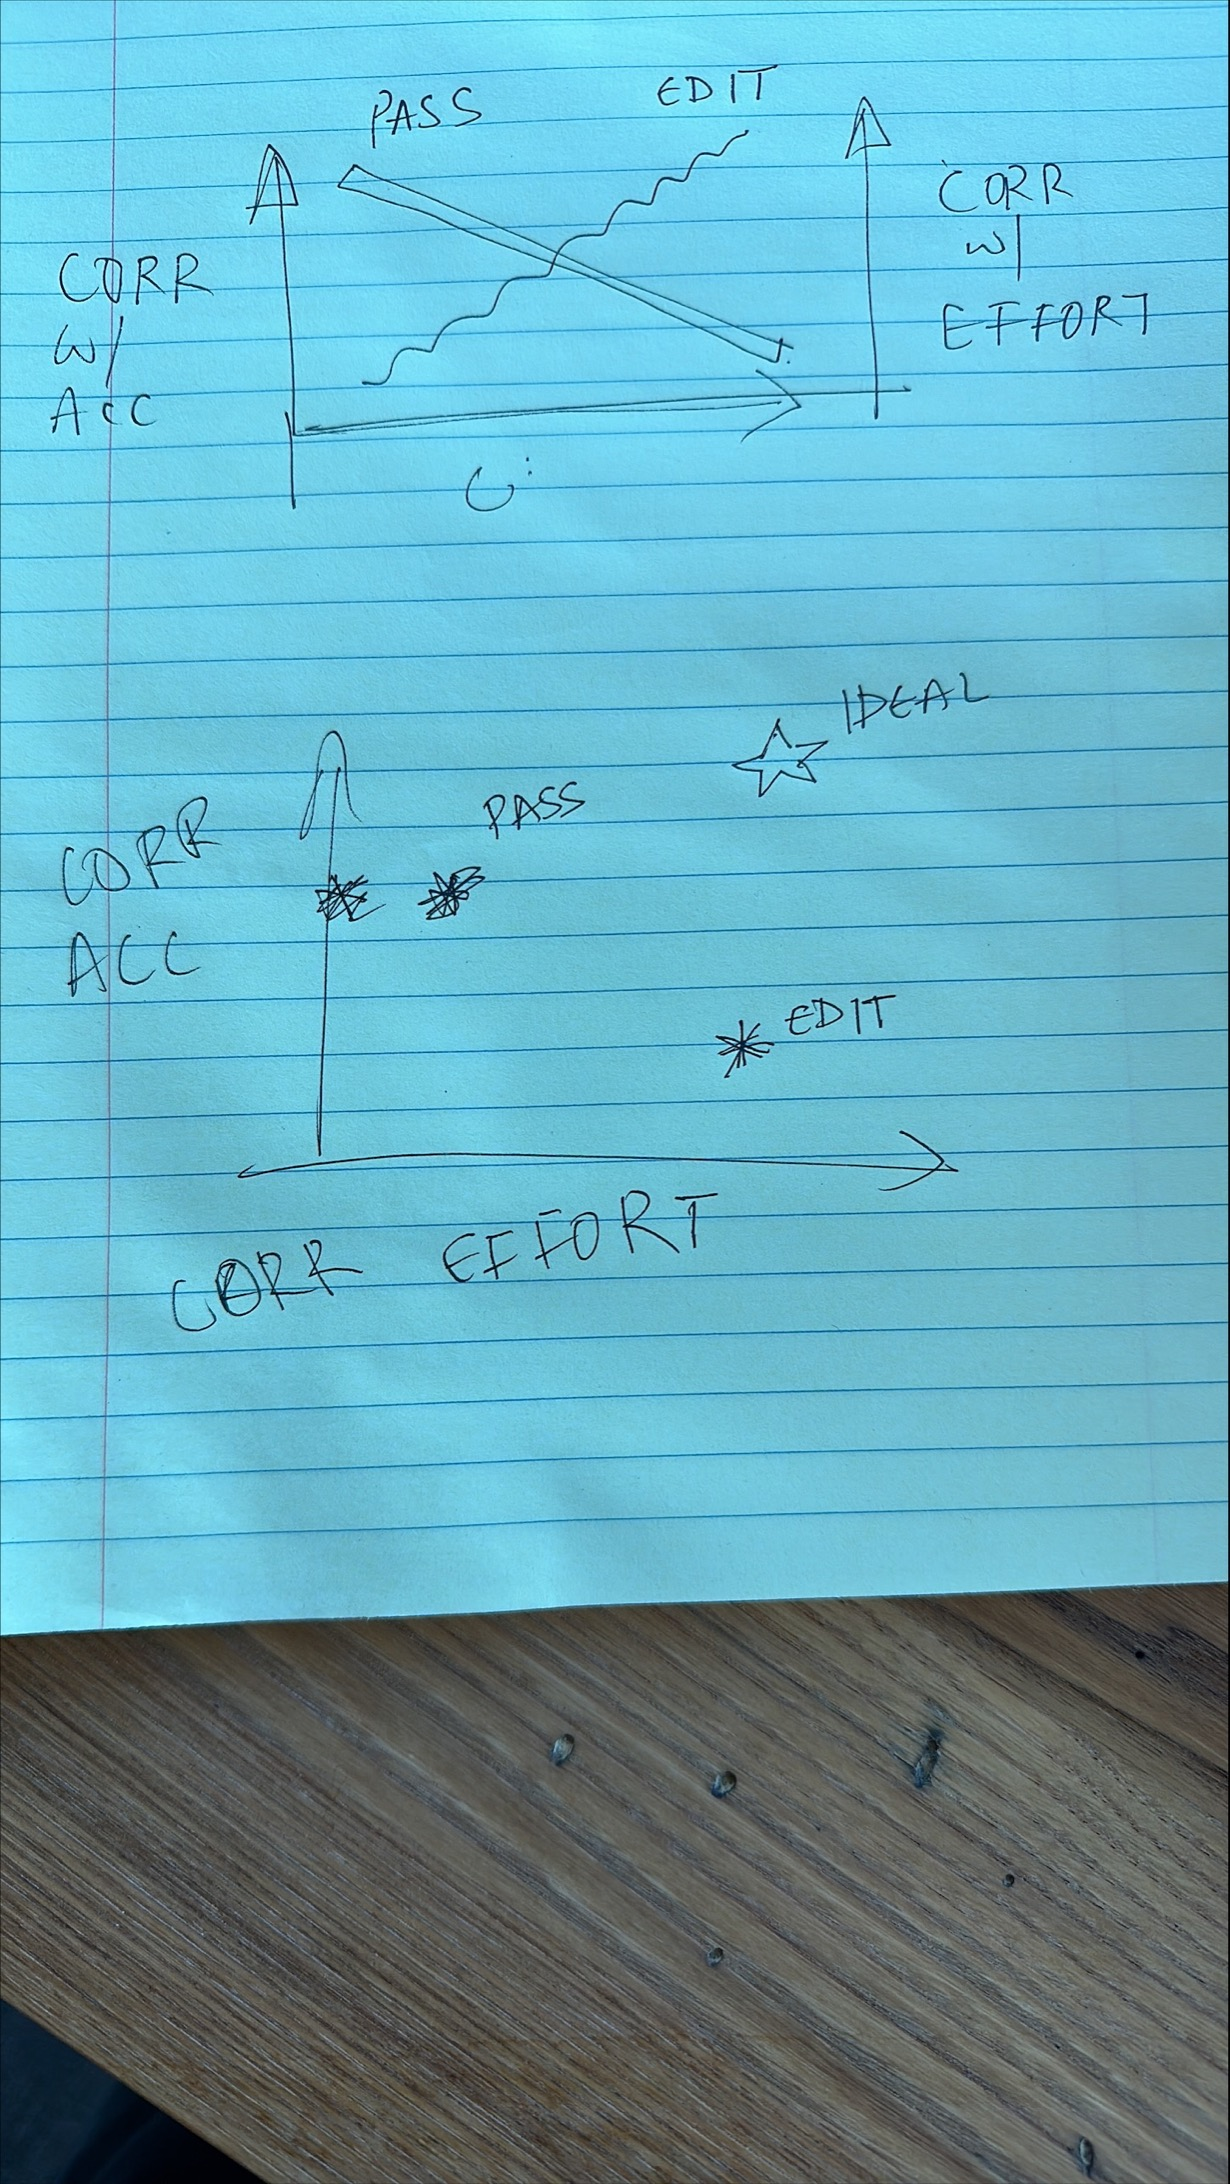}
    \caption{correlation between metrics and different dimensions of human preferences}
    \label{fig:my_label}
\end{figure}

\begin{figure}
    \centering
    \includegraphics[width=0.3\linewidth]{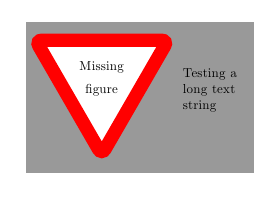}
    \caption{Scatter plot showing correlation between edit score and perceived effort for inidividual generations.}
    \label{fig:my_label}
\end{figure}

\begin{figure*}[t]
  \centering
  \begin{minipage}{.5\textwidth}
  \centering
  \includegraphics[width=\linewidth]{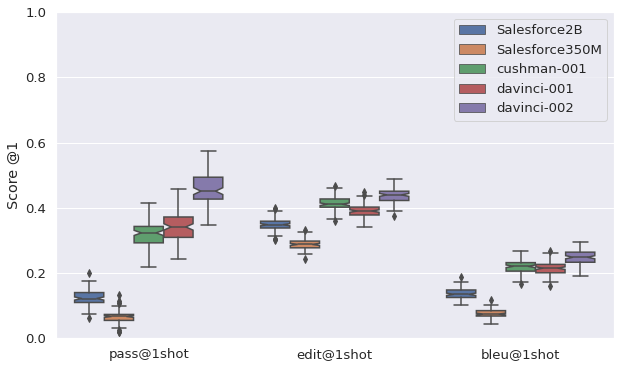}
  \captionof{figure}{Offline metric values per model}
  \label{fig:notchplots_at1}
\end{minipage}%
\begin{minipage}{.5\textwidth}
  \centering
  \includegraphics[width=\linewidth]{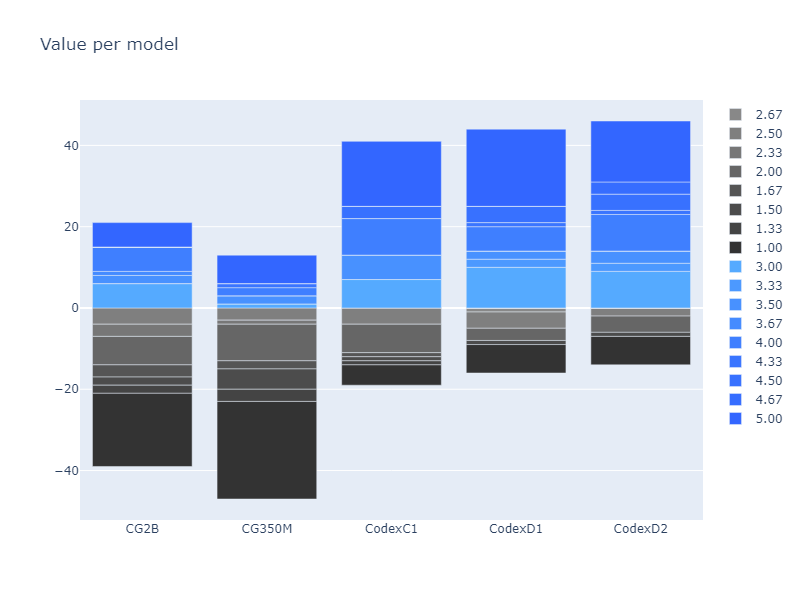}
  \captionof{figure}{Online human-judged value per model}
  \label{fig:notchplots_at10}
\end{minipage}
\end{figure*}

\begin{figure*}[t]
  \centering
  \begin{minipage}{.5\textwidth}
  \centering
  \includegraphics[width=\linewidth]{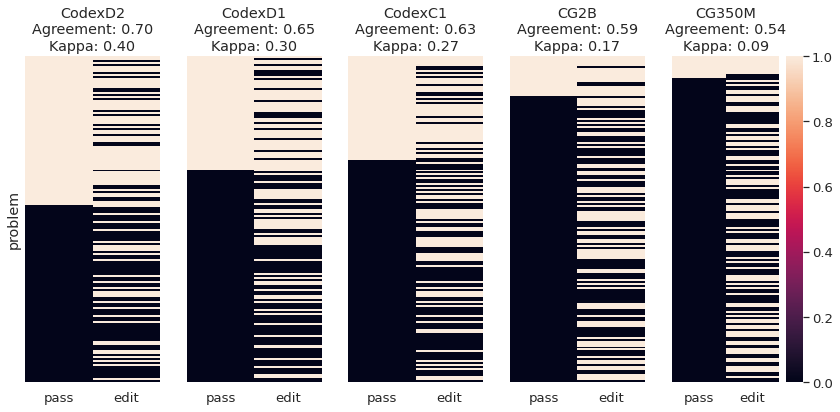}
  \captionof{figure}{Pass vs edit agreement over human-eval data}
  \label{fig:notchplots_at1}
\end{minipage}%
\begin{minipage}{.5\textwidth}
  \centering
  \includegraphics[width=\linewidth]{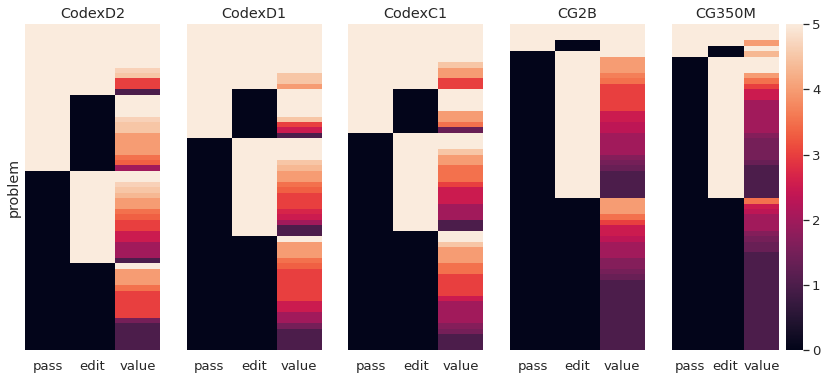}
  \captionof{figure}{Pass vs edit vs value over study data}
  \label{fig:notchplots_at10}
\end{minipage}
\end{figure*}

\begin{figure}[t]
     \centering
     \begin{subfigure}[b]{0.5\textwidth}
         \centering
         \includegraphics[width=\textwidth]{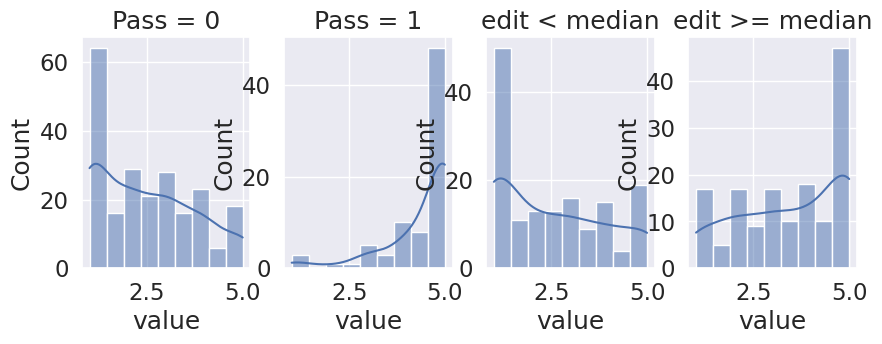}
         \caption{Both the functional correctness and similarity metric positively correlate with programmer's value -- suggestions that rate high on either offline metric are also rated higher in terms of value. However, functional correctness (left) shows a stronger correlations.\forough{Should we break these into separate figures rather than subfigures? That would allow us to reference specific figures in e.g., 4a.}
         \gagan{fix range of y-axis across hists; stack graphs together}
         }
         \label{fig:y equals x}
     \end{subfigure}
     \hfill

    \begin{subfigure}[b]{0.5\textwidth}
      \centering
          \includegraphics[width=\textwidth]{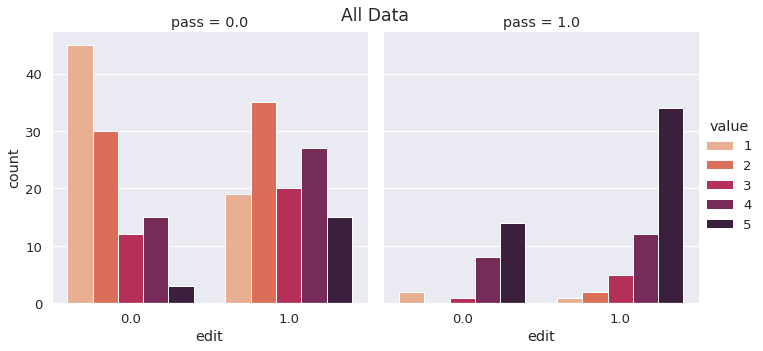}
          \caption{
          Inaccurate but useful code suggestions.
          Left histogram shows suggestions that fail unit but test may be deemed valuable by users. Circle shows a subset of these examples that can be captured by similarity metric plausibly because they are able to reward partial credit to code suggestions.
          % Pass doesn't give partial credit. Edit can when pass fails.
      \label{fig:valuebreakdown}} 
    \end{subfigure}
     \begin{subfigure}[b]{0.5\textwidth}
         \centering
         \includegraphics[width=\textwidth]{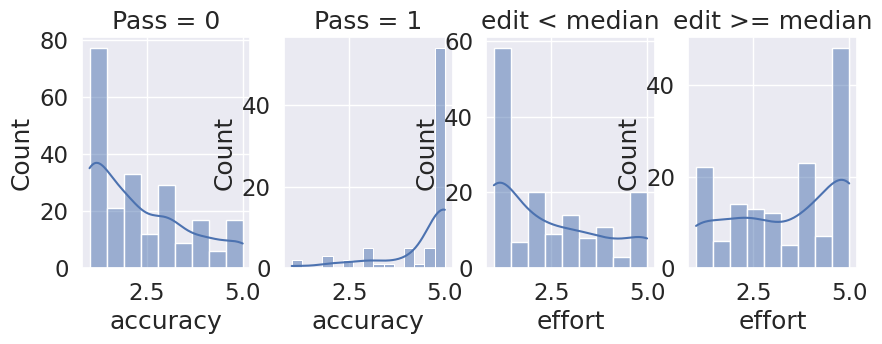}
         \caption{
         Perceived accuracy vs perceived effort.
         While pass is more correlated with perceived accuracy, edit is more correlated with perceived effort. \gagan{this figure needs to change. it should be a 2x2 grid. it needs to show that edit correlates more with effort than pass. and pass correlates more with accuracy than edit.}}
         \label{fig:five over x}
     \end{subfigure}
    
    \caption{(a) Correlation between metrics and human value. (b)  Inaccurate but useful code suggestions. (c) Correlation between metrics and perceived accuracy and effort.}
    \label{fig:three graphs}
\end{figure}

\begin{figure}
    \centering
    \includegraphics[width=\linewidth]{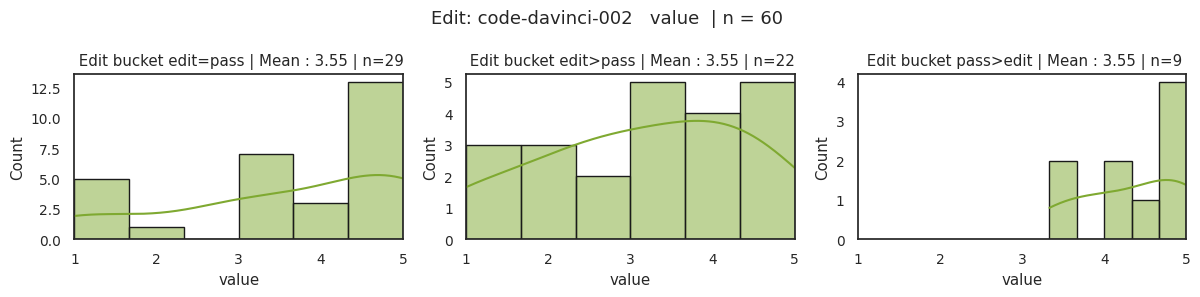}
    \caption{Our user study empirically confirms the scenario in Figure~\ref{fig:??} -- similarity metrics can help identify code suggestions that fail unit tests but are {\em highly} valuable to programmers. The circle indicates such instances for Davinci-2 on the HumanEval.
    % code suggestions that are rated as high value by subjects even when they fail the unit tests.
    \gagan{make the y-axis consistent and circle the second column with high value and tie it with figure 1; decrease width of each column, increase font size.}
    }
    \label{fig:my_label}
\end{figure}

\begin{figure*}[t]
  \centering
  \begin{subfigure}[b]{0.49\textwidth}
  \centering
  \includegraphics[width=\linewidth]{figures/notch_plots_at1.png}
  \caption{While results on the entire HumanEval dataset with the \passOne offline metric suggests that Davinci-2 is a significantly better model, similarity-based metrics find no difference between the top three models.}
  \label{fig:notchplots_at1}
\end{subfigure}%
\hfill
\begin{subfigure}[b]{0.49\textwidth}
  \centering
  \includegraphics[width=\linewidth]{figures/value_per_model_div_bar.png}
  \caption{Human judgements of perceived value, accuracy, and effort suggest no difference between the top three models. \gagan{Add accuracy and effort to this plot similar to the sub figure a; use same size as a; remove title}
  }
  \label{fig:notchplots_at10}
\end{subfigure}
\caption{Comparison of rankings of five state-of-art code generation models on three offline and online metrics.}
\end{figure*}

\begin{figure}[t]
    \centering
    \includegraphics[width=\linewidth]{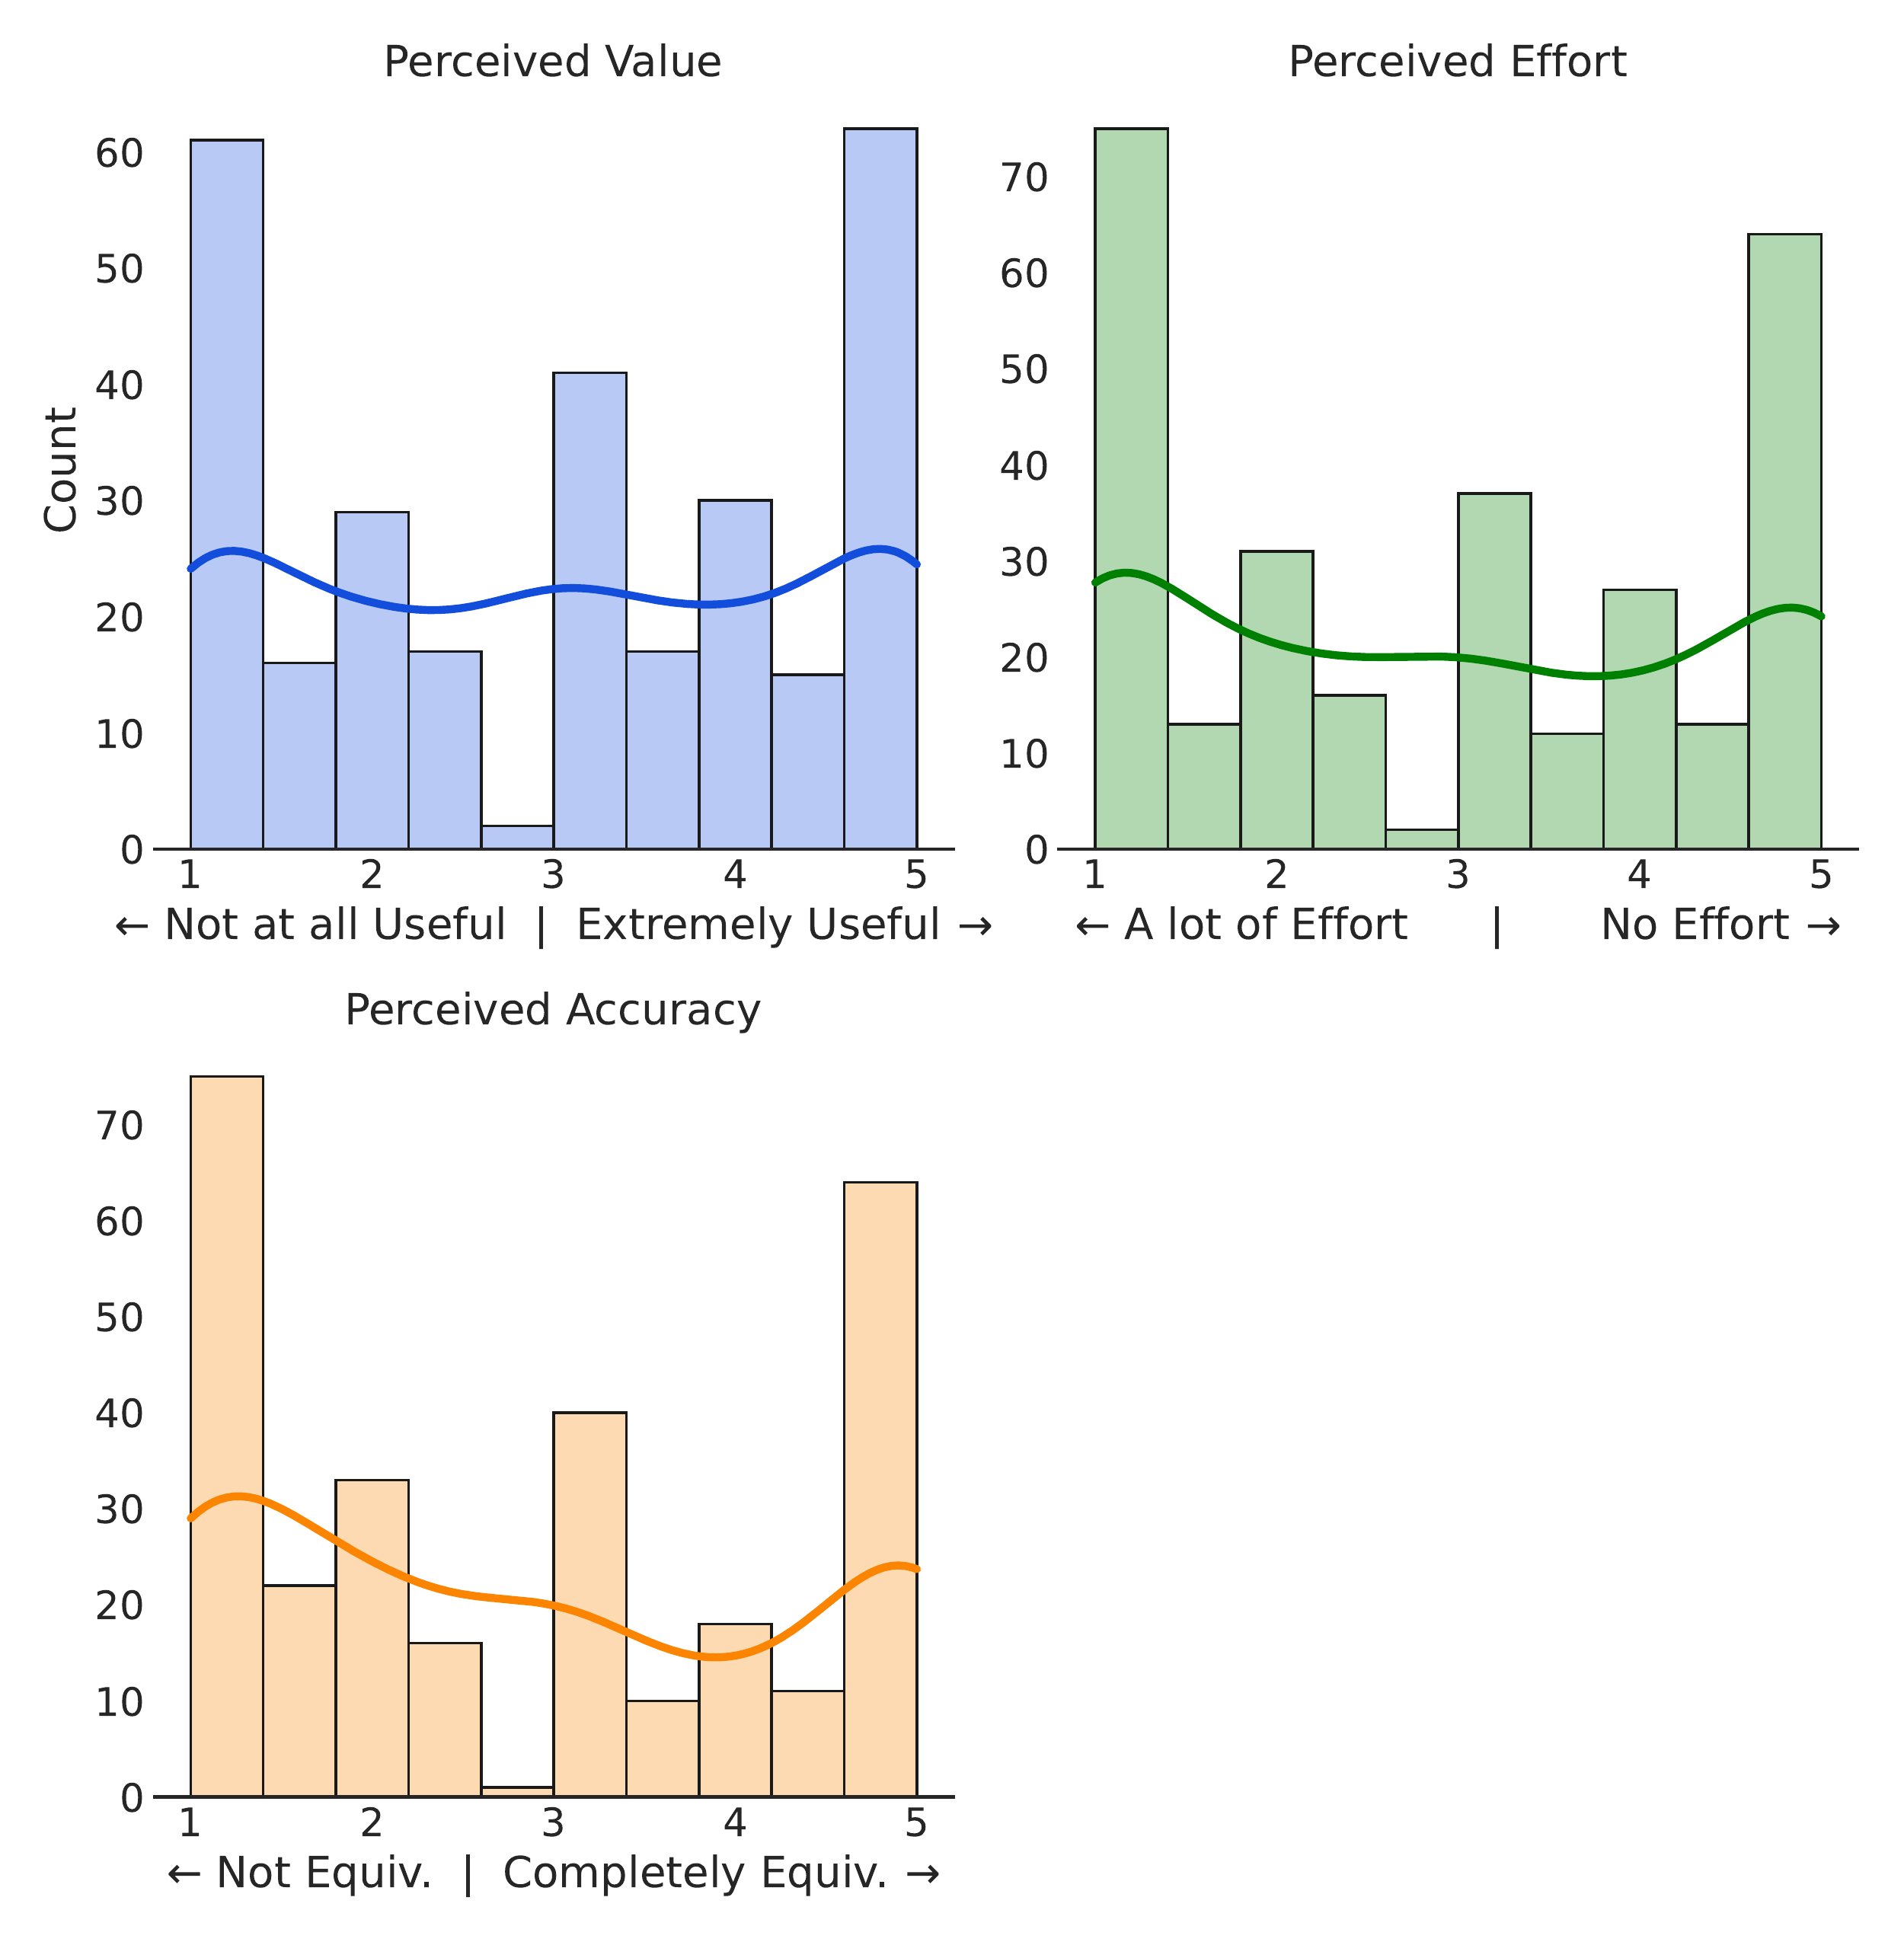}
    \caption{Distribution of programmers' judgements of perceived value, accuracy, and effort for code generations made by the Davinci-2 model, showing that they are highly correlated. We observe similar results for other models. \attention{TODO: update figure; increase font size.}}
    \label{fig:judgementdist}
\end{figure}
